# Supplementary material for: LLMs as On-demand Customizable Service
Source: arXiv:2401.16577 source file (2024-01-29)
Supplement: Supplementary file 1 [file appendix.tex]

\appendix

\section{Appendix}

%%keyboard applications~\cite{keyboard},

\subsection{Large Language Model (LLM) \& Prompts}Considerable progress has been made in the field of large language models, with notable applications including automatic news summarization~\cite{zhang2023benchmarking}, efficient healthcare research~\cite{sallam2023chatgpt}, software bug solving~\cite{surameery2023use}, and machine translation~\cite{jiao2023chatgpt}. %These examples highlight the remarkable capability of large language models to tackle complex tasks and provide practical solutions in real-world scenarios. 
Comparative studies have demonstrated the superiority of large language models over traditional models like BERT in certain tasks, while achieving comparable performance in others~\cite{zhong2023chatgpt}. Prompt engineering is an increasingly important skill set needed to effectively explore large language models (LLMs), some works in this direction are: chain of thought prompting~\cite{wei2023chainofthought}, self-consistency prompting~\cite{self-consistency-prompt}, synthetic prompting~\cite{shao2023synthetic}, generated knowledge prompting~\cite{liu2022generated}, and input-output prompting~\cite{ma2023fairnessguided}. Furthermore, research initiatives such as FrugalGPT~\cite{FrugalGPT-red-cost} have focused on leveraging LLMs in a more sustainable and efficient manner, achieving comparable performance to top-tier LLMs while significantly reducing costs. 

%We leverage the use of federated learning (FL) in our architecture. Prior research has explored the use of federated learning (FL)  in privacy-oriented natural language processing (NLP) applications, such as text intent classification~\cite{textfl}, high-quality language model training~\cite{largelang}, and medical systems~\cite{med1}. However, most of these studies are limited to specific application domains. In contrast, our proposed framework offers a unified platform that facilitates the investigation of diverse NLP applications in a shared environment, spanning a wide range of application domains.

\subsection{Continual Learning (CL):}

However, the existing research falls short in providing comprehensive solutions to address the challenges surrounding the availability and practical use of large language models (LLMs). It is evident that further research and innovative strategies are needed to overcome these limitations and fully unleash the power of LLMs in real-world applications.

 %These challenges are particularly crucial in resource-constrained environments, where the efficient utilization of LLMs is of utmost importance. Moreover, the exploration of prompt engineering techniques and cost-effective approaches for maximizing the potential of LLMs remains largely untapped. 
 
 %%related work federated learning
 %We leverage the use of federated learning (FL) in our architecture. Prior research has explored the use of federated learning (FL)  in privacy-oriented natural language processing (NLP) applications, such as text intent classification~\cite{textfl}, high-quality language model training~\cite{largelang}, and medical systems~\cite{med1}. However, most of these studies are limited to specific application domains. In contrast, our proposed framework offers a unified platform that facilitates the investigation of diverse NLP applications in a shared environment, spanning a wide range of application domains.
